# Supplementary material for: TeacherLM: Teaching to Fish Rather Than Giving the Fish, Language Modeling Likewise
Source: arXiv:2310.19019 source file (2024-07-16)
Supplement: Supplementary file 1 [file appendix.tex]

%\subsection{Training TeacherLM Hyperparameter}
%\input{table/TeacherLM.tex}
% \subsection{Comparison Experiment Hyperparameter}
% \subsection{Human Evaluation Details}

% Please rate the quality of explanations over the following aspects: (1) Fluency; (2) Consistency; (3) Factuality; (4) Sufficiency of Information; (5) Minimality; (6) Correlation; (7) Logical Coherence; (8) Overall Quality. We provide some instructions for your rating.

% \begin{enumerate}
%     \item Fluency

%     This measures whether the generated text has no formatting problems, capitalization errors, or ungrammatical sentences (e.g., fragments, missing components) that make the text difficult to read. The definitions of different scores are:
    
% \begin{itemize}
%     \item 10-9: The text is fluent, grammatically correct, error-free, and easy to read.
%     \item 8-7: The text contains minor grammatical, spelling, or capitalization errors, which do not impair comprehension.
%     \item 6-5: This text contains minor grammatical and spelling errors that slightly impair your understanding.
%     \item 4-3: This text contains significant grammatical and spelling errors that make the text difficult to read.
%     \item 2-1: The text has no meaning and is unreadable.
% \end{itemize}

%     \item Consistency
 
%     This evaluates the contextual consistency of the generated explanation, that is, whether there are logical contradictions or semantic incompleteness. The definitions of different scores are:

% \begin{itemize}
%     \item 10-9: The explanation has no logical contradiction, and the semantics are complete.
%     \item 8-7: There are a few logical contradictions in the explanation while the semantics are complete.
%     \item 6-5: There are some logical contradictions in the explanation or semantic coherence flaws.
%     \item 4-3: There are a lot of logical contradictions in the explanation, or there are semantic coherence flaws.
%     \item 2-1: The explanation is poorly logical and incoherent in context.
% \end{itemize}

%     \item Factuality
    
%     This measures whether the generated explanation aligns with the facts. You may use the internet to search for information to help you decide. The definitions of different scores are:
    
% \begin{itemize}
%     \item 10-9: There are no factual errors in the explanation.
%     \item 8-7: There are a few factual errors in the explanation, but they do not affect the final answer.
%     \item 6-5: There are factual errors in the explanation that may affect the reasoning of the answer.
%     \item 4-3: There are many factual errors in the explanation, which seriously affect the reasoning of the answer.
%     \item 2-1: The explanation is entirely unreliable.
% \end{itemize}

%     \item Sufficiency of Information
    
%     This measures whether the information in the explanations is sufficient for the answer. In other words, determine if you need to add new information to get this answer. The definitions of different scores are:

% \begin{itemize}
%     \item 10-9: The answer can be inferred without adding any new information.
%     \item 8-7: Some simple common sense information is missing in the explanation, which can be added or not, and does not affect the final answer.
%     \item 6-5: A key piece of information is missing from the explanation, and the answer cannot be deduced from the explanation alone.
%     \item 4-3: Two or more key pieces of information are missing, and the answer cannot be deduced from the explanation alone.
%     \item 2-1: All critical information is missing from the explanation.
% \end{itemize}
 
%     \item Minimality
    
%     This measures whether there is redundant information in the generated explanation, in other words, whether some sentences can be removed and the answer can still be obtained. The definitions of different scores are:

% \begin{itemize}
%     \item 10-9: No information in the explanation can be removed. Otherwise, the answer cannot be deduced.
%     \item 8-7: There is information in the explanation that is irrelevant to the final answer and can be removed.
%     \item 6-5: Less than half of the information in the explanation is irrelevant to the final answer and can be removed.
%     \item 4-3: More than half of the information in the explanation is irrelevant to the final answer and can be removed.
%     \item 2-1: All information in the explanation is irrelevant to the final answer and can be removed.
% \end{itemize}

%     \item Correlation
    
%     This measures how relevant the generated explanation is to the question and answer. The definitions of different scores are:
    
% \begin{itemize}
%     \item 10-9: All the explanation content is related to the question or answer.
%     \item 8-7: Most of the content in the explanation is related to the question or answer.
%     \item 6-5: About half of the content in the explanation is related to the question or answer.
%     \item 4-3: A small portion of the explanation is related to the question or answer.
%     \item 2-1: Nothing in the explanation is related to the question or answer.
% \end{itemize}
    
%     \item Logical Coherence
    
%     This measures whether the step-by-step part of the generated explanation has a logical sequence. For example, whether the logical order of the new explanation is more reasonable if Step1 and Step2 in the step-by-step part are replaced. The definitions of different scores are:
    
% \begin{itemize}
%     \item 10-9: The steps in the explanation are strongly sequential and cannot be reversed.
%     \item 8-7: The steps in the explanation are highly coherent, and changing the order will have a specific impact on the inference of the answer.
%     \item 6-5: The steps in the explanation are not coherent, and switching the order has little effect on the reasoning of the answer.
%     \item 4-3: The steps in the explanation are less coherent, and it may be better to reverse the order of some steps.
%     \item 2-1: The logical order of the steps in the explanation is completely reversed.
% \end{itemize}
    
%     \item Overall Quality
    
%     This measures the overall quality of the generated explanation judged by yourself. The definitions of different scores are:
    
% \begin{itemize}
%     \item 10-9: Very good.
%     \item 8-7: Good.
%     \item 6-5: Not bad.
%     \item 4-3: Poor.
%     \item 2-1: Very poor.
% \end{itemize}

% \end{enumerate}
